# Supplementary material for: Optimizing Ranking Systems Online as Bandits
Source: arXiv:2110.05807 source file (2021-10-12)
Supplement: Supplementary file 2 [file Appendix.tex]

%!TEX root = paper.tex
\appendix

\section{Proof of Theorem~\cref{th: regret}} 
\label{sec:proof of theorem}
\todo{Add more descriptions on the proof. More text and more equations.}
\if0 % CL: no space
\addtocounter{thm}{-1}
\begin{thm}
For  $\norm{\vw^*} \leq 1$ and any 
\begin{equation*}
%\label{eq:gamma}
\gamma \geq \sqrt{(m+d)\log(1+\frac{nk}{m+d}) + 2\log(n)} + \norm{\vw^*}, 
\tag{\cref{eq:gamma}}
\end{equation*}
we have 
\begin{equation*}
%	\label{eq:regret bound}
	R_{\eta}(n) \leq 
2\gamma \sqrt{{2nK(d+m)\log{(1+\frac{nK}{m+d})}}}
	+ 1.	
\tag{\cref{eq:regret bound}}	
\end{equation*}
\end{thm}
\fi

%We first define some notations. 
We write $\vw^* = [\vtheta^{*T}, \vbeta^{*T}]^T$. 
Given a ranked list $\cR$ and $a = \cR(i)$, we write $\vphi_a  = [\vomega_{a}^T, \vz_{a}^T]^T$.\footnote{With $\vphi_a$ and $\vw^*$ notations, $\cascadehybrid$ can be viewed as an extension of $\cascadelsb$, where two submodular functions instead of one are used in a single algorithm. 
Note that the linear function can be viewed as a special case of submodular functions. }
We write $\vOt = \vI_{m+d} + \sum_{i=1}^{t-1}\sum_{a\in\cO_i} \vphi_a \vphi_a^T$ as the collected features in $t$ steps, and  $\cH_t$ as the collected features and clicks up to step $t$.
We write $\cR^i = (\cR(1), \ldots, \cR(i))$.  
Then, the confidence bound in \cref{eq:cb} on the $i$-th item in $\cR$ can be re-written as:  
\begin{equation}
\label{eq:new cb}
	s(\cR^i) = \vphi_{\cR(i)}^T \vOt^{-1} \vphi_{\cR(i)}. 
\end{equation}
Let $\Pi(\cD) = \cup_{i=1}^L\Pi_i(\cD)$ be the set of all ranked lists of $\cD$ with length $[L]$, and $\kappa: \Pi(\cD) \rightarrow [0, 1]$ be an arbitrary list function. 
For any $\cR \in \Pi(\cD)$ and any $\kappa$, we  define 
\begin{equation}
	\label{eq:new f}
	f(\cR, \kappa) = 1 - \prod_{i=1}^{|\cR|} (1-\kappa(\cR^i)).
\end{equation}
We define upper and lower confidence bound, and  $\kappa$ as: 
\begin{equation}
\label{eq:ucb lcb}
\begin{split}
	u_t(\cR) ={}& \text{F}_{[0, 1]}[\vphi_{\cR(l)}^T\hat{\vw}_t + s(\cR^l)]  \\
	l_t(\cR) = {}&\text{F}_{[0, 1]}[\vphi_{\cR(l)}^T\hat{\vw}_t - s(\cR^l)] \\
	\kappa(R) = {}&\vphi_{\cR(l)}^T\vw^*, 
	\end{split}
\end{equation}
where $l = |\cR|$ and  $\text{F}_{[0,1]}[\cdot] =  \max(0, \min(1, \cdot))$. 
With the definitions in \cref{eq:ucb lcb}, $f(\cR, \kappa) = r(\cR, \valpha)$ is the reward of list $\cR$.

\begin{proof}
Let $g_t = \{ l_t(\cR) \leq \kappa(\cR) \leq u_t(\cR), \forall \cR \in \Pi(\cD)\}$ be the event that the attraction probabilities are bounded  by the lower and upper confidence bound, and $\bar{g}_t$ be the complement of $g_t$. 
We have 
\begin{equation}
\label{eq:regret to f}
\begin{split}
	\expect{\eta r(\cR^*, \valpha) - r(\cR_t, \vA_t)} & =	\expect{\eta f(\cR^*, \kappa) - f(\cR_t, \kappa)} \\
	&\stackrel{(a)}{\leq} P(g_t) \expect{\eta f(\cR^*, \kappa) - f(\cR_t, \kappa)} + P(\bar{g}_t) \\
	&\stackrel{(b)}{\leq} P(g_t) \expect{\eta f(\cR^*, u_t) - f(\cR_t, \kappa)} + P(\bar{g}_t)  \\
	&\stackrel{(c)}{\leq} P(g_t) \expect{ f(\cR_t, u_t) - f(\cR_t, \kappa)} + P(\bar{g}_t),  
\end{split}
\end{equation}
where $(a)$ holds because $\expect{\eta f(\cR^*, \kappa) - f(\cR_t, \kappa)} \leq 1$,  $(b)$ holds because under event $g_t$ we have $f(\cR, l_t) \leq f(\cR, \kappa) \leq f(\cR, u_t)$, $\forall \cR \in \Pi(\cD)$, and $(c)$ holds by the definition of the $\eta$-approximation, where we have  
\begin{equation}
	\eta f(\cR^*, u_t) \leq  \max_{\cR \in \Pi_K(\cD)} \eta f(\cR, u_t) \leq f(\cR_t, u_t). 
\end{equation}
By the definition of the list function $f(\cdot, \cdot)$ in \cref{eq:new f}, we have 
{\footnotesize
\begin{equation}
\begin{split}
%\mbox{}\hspace*{-13mm}
f(\cR_t, u_t) - f(\cR_t, \kappa) 
&= \prod_{k=1}^{K} (1- \kappa(\cR_t^k)) -  \prod_{k=1}^{K} (1- u_t(\cR_t^k)) 
\\
	&\stackrel{(a)}{=} \sum_{k=1}^{K} \!\!\left[ \prod_{i=1}^{k-1} (1- \kappa(\cR_t^i)) \right] \!\!(u_t(\cR_t^k) - \kappa(\cR_t^k))\!\!
	\left[ \prod_{j=k+1}^{K} (1- u(\cR_t^j)) \right]   
\\
	&\stackrel{(b)}{\leq}  \sum_{k=1}^{K}\!\! \left[ \prod_{i=1}^{k-1} (1- \kappa(\cR_t^i)) \right] \!\!(u_t(\cR_t^k) - \kappa(\cR_t^k)),
\end{split}
\end{equation}}%
where $(a)$ follows from Lemma 1 in~\citep{zong16cascading} and $(b)$ is because of the fact that $0\leq \kappa(\cR_t) \leq u_t(\cR_t) \leq 1$. 
We then define the event $h_{ti} = \{\text{item } \cR_t(i) \text{ is observed} \}$, where we have $\expect{\ind{h_{ti}}} = \prod_{k=1}^{i-1} (1- \kappa(\cR_t^k))$.
For any $\cH_t$ such that $g_t$ holds, we have 
\begin{equation}
\label{eq:f to sqrt}
\begin{split}
 	&{}    \expect{f(\cR_t, u_t) - f(\cR_t, \kappa) \mid \cH_t}  \\
	&\leq \sum_{i=1}^K \expect{\ind{h_{ti}} \mid \cH_t }(u_t(\cR_t^i) - l_t(\cR_t^i))  \\
	&\stackrel{(a)}{\leq} 2\gamma \expect{\ind{h_{ti}} \sum_{i=1}^{K}\sqrt{s(\cR_t^i)}   \mid \cH_t}  \\
	&\stackrel{(b)}{\leq} 2\gamma \expect{\sum_{i=1}^{\min(K, c_t)}\sqrt{s(\cR_t^i)}   \mid \cH_t},  
\end{split}	
\end{equation}
where inequality $(a)$ follows from the definition of $u_t$ and $l_t$ in \cref{eq:ucb lcb}, and inequality $(b)$ follows from the definition of $h_{ti}$.
%inequality $(b)$ follows from the definition of $u_t$ and $l_t$ in \cref{eq:ucb lcb}, and the definition of $h_{ti}$. 
Now, together with \cref{eq:scaled regret,eq:regret to f,eq:f to sqrt}, we have 
\begin{equation}
\label{eq:proof cumulative regret}
\begin{split}
	 	R_{\eta}(n)& = \sum_{t=1}^{n}\expect{\eta r(\cR^*, \valpha) - r(\cR_t, \vA_t)  }  \\
	 &\leq  \sum_{t=1}^{n} \left[ 2\gamma  \expect{\sum_{i=1}^{\min(K, c_t)}\sqrt{s(\cR_t^i)}   \mid g_t} P(g_t) 
	 	 + P(\bar{g}_t) 
	 \right] \\ 
	 &\leq     2\gamma  \expect{\sum_{t=1}^{n}\sum_{i=1}^{K}\sqrt{s(\cR_t^i)} }
	 + \sum_{t=1}^{n}p(\bar{g}_t).  
\end{split}
\end{equation}
For the first term in \cref{eq:proof cumulative regret}, we have
\begin{equation}
\begin{split}
\label{eq:to det}
	&\sum_{t=1}^{n}\sum_{i=1}^{K}\sqrt{s(\cR_t^i)}
	\stackrel{(a)}{\leq} \sqrt{nK \sum_{t=1}^{n}\sum_{i=1}^{K}s(\cR_t^i)} 
	\stackrel{(b)}{\leq} 
	\sqrt{nK 2\log det(\vO_t) },  
\end{split}	
\end{equation}
where inequality $(a)$ follows from the Cauchy-Schwarz inequality and $(b)$ follows from Lemma 5 in~\citep{yue-2011-linear}. 
Note that $\log det(\vO_t) \leq (m+d) \log(K(1+n/(m+d)))$ and together with \cref{eq:to det}:
\begin{equation}
\label{eq:to log}
\mbox{}\hspace*{-2mm}
\sum_{t=1}^{n}\sum_{i=1}^{K}\sqrt{s(\cR_t^i)} 
	\leq 
	\sqrt{2nK(m+d)\log(K(1+\frac{n}{m+d}))  }. 
\hspace*{-2mm}\mbox{}
\end{equation}
For the second term in \cref{eq:proof cumulative regret}, by Lemma 3 in~\citep{Hiranandani2019CascadingLS}, we have $P(\bar{g}_t) \leq 1/n$ for any $\gamma$ satisfies \cref{eq:gamma}. 
\if0
\begin{equation}
	\gamma \geq \sqrt{(m+d)\log(1+\frac{nk}{d}) + 2\log(n)} + \norm{\vw^*}. 
\end{equation}
\fi
Thus, together with \cref{eq:proof cumulative regret,eq:to det,eq:to log}, we have 
\begin{equation*}
		R_{\eta}(n) \leq 2\gamma\sqrt{2nK(m+d)\log(1+\frac{nK}{m+d}) }  +1. 
\end{equation*}
That concludes the proof of Theorem~\cref{th: regret}.
\end{proof}

\if0 % delete due to space limitaion
\section{Derivation of $\cascadehybrid$}
\label{sec:deviation of cascadehybrid}

In this section, we derive the closed form solution to $\cascadehybrid$. 
Let $\vOmegat \in \mathds{R}^{t \times d}$ be the collected topic gains in previous $t$ steps. 
Let $\vZt \in \mathds{R}^{t \times m}$ be the collected relevance features in previous $t$ steps. 
Let $\vQt = [\vOmegat; \vZt] \in \mathds{R}^{t \times (d+m)}$. 
Let $\vb_t \in \{0, 1\}^{t}$ be the collected click feedback in previous $t$ steps, where $0$ indicts non-click and $1$ indicts click. 
We write the estimate parameter at step $t$ as $\vw_t$. 
Thus, given a ranked list $\cR$, the estimated attraction probability of item in the $i$th position by $\cascadehybrid$ is
\begin{equation}
	\alphabar(\cR) = \vphi_{\cR(i)}\vwt, 
\end{equation}
where we define $\vphi_{\cR(i)} = [\vomega_{\cR(i)}^T, \vz_{\cR(i)}^T]^T$for simplicity. 
For simplicity, we write the user preference as: $\vw = [\vtheta^{*T}, \vbeta^{*T}]^T$. 

In $\cascadehybrid$, the maximize the likelihood is used to estimate $\vw$ and thus we  have the loss function
\begin{equation}
	\mathcal{L} = \norm{\vb_t - \vQt \vw_t}^2 . 
\label{eq:l2loss}
\end{equation}
This problem can be solved in a closed form as follows: 
\begin{equation}
	\vw_t = \left[\vQt^T\vQt\right] ^{-1} \vQt^T\vb_t. 
\end{equation}
We can compute the matrix inverse as follows: 
\begin{equation}
\begin{split}
[\vQt^T\vQt] ^{-1} ={}& 
	\begin{bmatrix}
		\vOmegat^T \vOmegat & \vOmegat^T \vZt \\
		\vZt^T \vOmegat & \vZt^T \vZt
	\end{bmatrix}^{-1} \\
	 ={}&
	 \begin{bmatrix}
	 \vH_t^{-1} & -\vH_t^{-1}\vB_t\vM_t^{-1} \\
	-\vM_t^{-1}\vB_t\vH_t^{-1} & \vM_t^{-1} + \vEt
	 \end{bmatrix},  
\end{split}	 
\label{eq:matrix inverse}
\end{equation}
where $\vB_t = \vOmegat^T \vZt $, $\vM_t =  \vZt^T \vZt$, $\vH_t = \vOmegat^T \vOmegat - \vB_t\vM_t^{-1}\vB_t^T$ and we write $\vEt = \vM_t^{-1}\vB_t^T\vH_T^{-1}\vB_t\vM_t^{-1}$ for short . 
The first equality is due to basic matrix multiplications; the second one is based on matrix block-wise inversion~\citep{golub-1996-matrix}. 

Then, we compute $\vthetahat_t$ and $\hat{\vbeta}_t$. 
Together with \cref{eq:l2loss} and \cref{eq:matrix inverse}, we compute the estimated parameter as follows: 
\begin{equation}
\begin{split}
\mbox{}\hspace*{-2mm}
	\begin{bmatrix}
	\vthetahat_t \\
	\hat{\vbeta}_t
	\end{bmatrix} ={}&  \left[\vQt^T\vQt\right] ^{-1} \vQt^T\vb_t \\
							={}& 
							\begin{bmatrix}
							\vH_t^{-1} & -\vH_t^{-1}\vB_t\vM_t^{-1} \\
							-\vM_t^{-1}\vB_t^T\vH_t^{-1} & \vM_t^{-1} + 
							\vEt
							\end{bmatrix}  
							\begin{bmatrix}
								\vOmegat^T\vb_t  \\
								\vZt^T\vb_t 
							\end{bmatrix}
							 \\
						={}&
						\begin{bmatrix}
						\vH_t^{-1} \vOmegat^T\vb_t -\vH_t^{-1}\vB_t\vM_t^{-1}  \vZt^T\vb_t  \\
							-\vM_t^{-1}\vB_t\vH_t^{-1} \vOmegat^T\vb_t + \vM_t^{-1} \vZt^T\vb_t + \vEt \vZt^T\vb_t 
						\end{bmatrix} .
\end{split}						
\end{equation}
Letting $\vy_t = \vZt^T \vb_t$, $\vu_t = \vOmegat \vb_t - \vB_t\vM_t^{-1} \vy_t$, we have the following closed forms: 
\begin{equation}
		\vthetahat_t =  \vH_t^{-1}\vu_t, \quad
	\hat{\vbeta}_t =  \vM_t^{-1}(\vy_t - \vB_t^T \hat{\vtheta_t}).
\end{equation}
The attraction probability of  an item with context $\{\vomega_{a}, \vz_a\}$ at step $t$ can be estimated as: 
\begin{equation}
		\tilde{\alpha}_{t, a} = \vomega_{a} \vthetahat_t + \vz_a \hat{\vbeta}_t. 
\end{equation}
Analogizing our estimator to the $\linucb$~\citep{li2010contextual}, we compute the confidence interval of the estimator at step $t$ as follows: 
\begin{equation}
\begin{split}
	s_{t, a} = {} &
	[\vomega_a^T, \vz_a^T]^T\left[\vQt^T\vQt\right] ^{-1} \begin{bmatrix}
	\vomega_a \\
	\vz_a 
	\end{bmatrix} \\
	= {} & \vomega_a^T\vH_t^{-1}\vomega_a - 2\vomega_a^T\vH_t^{-1}\vB_t\vM_t^{-1}\vz_a + \\
	&\quad \vz_a \vM_t^{-1} \vz_a + 
	\vz_a \vM_t^{-1}\vB_t^T\vH_t^{-1}\vB_t \vM_t^{-1} \vz_a.
\end{split}
\end{equation} 
Finally, we reach to the closed form of our \ac{UCB} estimator on item $a$: $\mu_{t, a} = \tilde{\alpha}_{a}  + \gamma \sqrt{s_{t, a}}$. 
\fi

\if0
\section{Notation}
\label{sec:notation}

\begin{table}
	\caption{Notation used in this paper.}
	\label{tb:notation}
	\begin{tabular}{p{0.2\columnwidth} p{0.65\columnwidth}}
		\toprule	
		\bf Notation & \bf Description \\
		\midrule
		$L$ & Number of items\\
		$[n]$ & $[1, \ldots, n]$ \\
		$\cD$ & Item set $\cD= [L]$\\
		$K$ & Number of positions $K \leq L$\\
		$\Pi(\cD)$ & Set of whole permutation of $K$ items from $\cD$  \\
		$\cR $ & Ranked list $\cR \in \Pi(\cD)$ \\ 
		$\cR(i)$ & Item at the $k$-th position \\
		$\cR^{-1}(i)$ & Position of item $i$ in $\cR$ \\ 
		$\alpha(\cR(i))$ & Attraction probability of $\cR(i)$, $\valpha \in [0,1]^L$\\ 
		$\cR_t$ & Displayed list at step $t$ \\ 
		$A_t$ & Attraction indicator at step $t$, 	$A_t \in \{0, 1\}^L$ \\
		$c_t$ & Click: $\vc_t \in \{0, 1\}^K$ \\
		$r(\cR_t, A_t)$ & Reward: $r(\cR_t) = 1 - \prod_{k=1}^{K} (1-A_t(\cR_t(k)))$ \\
		$m$ & Number of relevance features \\ 
		$d$ & Number of topics \\
		$\vz_i$  & Relevance feature: $\vz_i \in \real^{m}$ \\
		$\vx_i$ & Topic coverage of item $i$: $\vx_i \in \real^{d}$ \\ 
		$\vbeta^*$ & Relevance parameter: $\vbeta^* \in \real^{m}$ \\
		$\vtheta^*$ & Topic preference:  $\vtheta^* \in \real^{d}$ \\ 
		$\omega(\vx_{\cR_t(i)} | \cR_t(i))$ & Topic coverage gain of $\cR_t(i)$ \\ 
		$\alpha(\cR_t(i))$ & $\alpha(\cR_t(i)) = \vz_i^T \vbeta^* +\omega(\vx_{\cR_t(i)} | \cR_t(i))^T, \vtheta^*$ \\ 
		\bottomrule
	\end{tabular}
\end{table}
\fi
